# Supplementary material for: Simple and Powerful Architecture for Inductive Recommendation Using Knowledge Graph Convolutions
Source: arXiv:2209.04185 source file (2022-09-13)
Supplement: Supplementary file 1 [file A_synthetic_dataset.tex]

Recent research have shown that the popularity bias negatively affect the recommendations made for users~\cite{kowald2020unfairnessmusic, abdollahpouri2019unfairness}.
Specifically, users that are not as interested in popular or mainstream items still get recommendations for popular items; but as evaluation metrics are based on the average user, experiment still show recommenders that make popularity based recommendations usually perform well in the average case~\cite{cremonesi2010topnperformance,bellogin2017statisticalbias,ji2020revisitpopularitybias}.
Moreover, a focus on explainable AI and recommender systems using \gls{kg} have gained traction~\cite{ma2019jointlyexplainablerules,wang2019explainableknowledgegraphkprn}, but the evaluation of these explanations often requires user studies that can be time consuming~\cite{li2020surveyexplainable}. 

To overcome these problems, we create a synthetic dataset where user ratings adhere to explainable rules defined on a per-user basis and follow an item-rating distribution matching a predefined popularity bias.
The approach to define preference rules for users is similar to the one described in~\cite{balog2019transparentdataset}, but instead of working with tags we use patterns over a \gls{kg}. 

We define two types of constructs, patterns and rules.
A pattern is a sequence of transitions in the \gls{kg} that can describe movies.
Formally we define a pattern of length $k$ as $p=\{\relation_1\entity_1,\relation_2\entity_2, \ldots, \relation_k\entity_k\}$, s.t. $(\entity_{j-1},\relation_j, \entity_j)\in \graph$ for all $2\leq j\leq k$.
In this context $P$ refers to the set of all pattern combinations.
The patterns applicable for an item $\rec$ are defined as $P_\rec = \{p \pipe p\in P \text{ and } (\rec,\relation_1, \entity_1)\in \graph\}$. 

A rule identifies a set of items that a user likes, defined as a sequence $r= \{(\neg)p, (\neg)p, \ldots \}$, where $(\neg)$ indicates that some rules can optional contain negation of patterns (e.g., movies that are not of genre drama).
Intuitively it means that an item either has the pattern in the list or does not have the pattern, for example, a user likes an item if it has pattern A and not pattern B. 
The set of items matching a rule is $ symbol = \{\rec \pipe p\in P_\rec, \: \forall p \in r\text{ and } \neg p \notin P_\rec, \: \forall \neg p \in r \}$, where $r$ is a rule and $\rec{\in}\recs$ is an item.  
For a rule to be valid, the set of items matching the rule must be non-empty and if the rule contains any not patterns, then the rule where these patterns are negated (i.e., $\neg(\neg p) = p$) must be non-empty.
The latter part ensures that all patterns in the rule affects which items matches the rule. 

We define X rule templates where the italicized variable can be replaced with an entity in the \gls{kg} of same type. 
E.g., a rule could be user likes item, if item has the director 'Christopher Nolan' and the genre 'Heist Film'. 
Those rules can be generated from the following rule templates"
\begin{enumerate}
    \item user likes item, if item has \textit{director}.
    \item user likes item, if item has \textit{director} and \texttt{genre}. 
    \item user likes item, if item has \textit{pattern A} and not \texttt{pattern B}.
\end{enumerate}

Given the rules, to generate ratings, we follow these three steps: \begin{enumerate*}[label=(\roman*)]
  \item generate user templates given real users, as seen on lines 1-7 in \autoref{algo:synthetic_users};
  \item assign users to rules given a user templates on lines 8-13; and
  \item generate ratings for each user based on rules on lines 14-19.
\end{enumerate*}

Finally, we define a set of popular items (based on which items are popular in the real dataset) and for each user we add a portion of likes relationships to those items so to reach the given popularity bias $\beta$.
We performed different experiments showing that we can reach the desired popularity bias.
\clearpage

\begin{algorithm}[thb!]
    \SetKwInOut{Input}{input}\SetKwInOut{Output}{output}
    \Input{\gls{kg} $\graph$, real users, rule templates, number of user templates $n$, number of synthetic users $m$, number of rules per synthetic user $k$, popularity bias $\beta$}
    \Output{Set of user-item pair representing item liked by user}
    \BlankLine
    
    Initialize dictionary mapping user to rules $\users_t$;
    
    \For{$i := 0$ \KwTo $n$}{
        $\user :=$ sampled user from real user\;
        \For{rule in rule templates}{
            $\rec :=$ sampled liked item from $\user$\;
            $r :=$ Query \gls{kg} for rules matching $i$ given rule template\;
            Add $k$ rules from $r$ to $\users_t(\user)$\;
        }
        
    }
    
    Initialize dictionary mapping rule to synthetic user ids $R_s$\;
    \For{$i := 0$ \KwTo $m$}{
        $\user :=$ sample random user from $\users_t$\;
        $R :=$ Sample $k$ rules from $\users_t(\user)$\;
        
        \ForEach{$r$ in $R$}{
            Append $i$ to $R_s(r)$\;
        }
    }
    
    Initialize set empty set of ratings $I$\;
    \ForEach{rule in $R_s$}{
        Query \gls{kg} for items matching rule\;
        
        \ForEach{user in $R_s(rule)$}{
            \ForEach{item matching rule}{
                Add user-item tuple to $I$\;
            }
        }
    }
    Add popularity bias  $\beta$ to $I$\;
    \Return{$I$}  \;
    
    \caption{Generate synthetic users}\label{algo:synthetic_users}
\end{algorithm}

\clearpage
