# Supplementary material for: Simple and Powerful Architecture for Inductive Recommendation Using Knowledge Graph Convolutions
Source: arXiv:2209.04185 source file (2022-09-13)
Supplement: Supplementary file 2 [file C_tables.tex]

% Please add the following required packages to your document preamble:
% \usepackage{multirow}
\begin{table*}[]
\resizebox{\linewidth}{!}{%
\begin{tabular}{|c|l|r|r|r|}
\hline
\multicolumn{1}{|r|}{}        & \multicolumn{1}{r|}{} & \textbf{TopPop}                 & \textbf{BPR-MF}                 & \textbf{KGAT}                   \\ \hline
\multirow{4}{*}{Ml-s}         & ndcg@20               & *0.108{\textpm}0.001            & \underline{0.133{\textpm}0.002} & \textbf{0.144{\textpm}0.002}    \\ \cline{2-5} 
                              & recall@20             & *0.142{\textpm}0.001            & \underline{0.183{\textpm}0.003} & \textbf{0.205{\textpm}0.003}    \\ \cline{2-5} 
                              & precision@20          & *0.052{\textpm}0.001            & \textbf{0.065{\textpm}0.000}    & \underline{0.065{\textpm}0.001} \\ \cline{2-5} 
                              & cov@20                & *0.021{\textpm}0.001            & \textbf{0.610{\textpm}0.038}    & \underline{0.512{\textpm}0.004} \\ \hline
\multirow{4}{*}{Synthetic-1m} & ndcg@20               & *0.699{\textpm}0.004            & \textbf{0.801{\textpm}0.001}    & \underline{0.788{\textpm}0.003} \\ \cline{2-5} 
                              & recall@20             & *0.009{\textpm}0.000            & \textbf{0.012{\textpm}0.000}    & \underline{0.011{\textpm}0.000} \\ \cline{2-5} 
                              & precision@20          & *0.694{\textpm}0.004            & \textbf{0.801{\textpm}0.001}    & \underline{0.787{\textpm}0.004} \\ \cline{2-5} 
                              & cov@20                & *0.006{\textpm}0.000            & \textbf{0.767{\textpm}0.006}    & \underline{0.409{\textpm}0.018} \\ \hline
\multirow{4}{*}{Synthetic-16} & ndcg@20               & *0.0064{\textpm}0.000            & \textbf{0.0080{\textpm}0.000}    & \underline{0.0073{\textpm}0.000} \\ \cline{2-5} 
                              & recall@20             & *0.0094{\textpm}0.000            & \textbf{0.0123{\textpm}0.000}    & \underline{0.0113{\textpm}0.000} \\ \cline{2-5} 
                              & precision@20          & *0.0036{\textpm}0.000            & \textbf{0.0042{\textpm}0.000}    & \underline{0.0040{\textpm}0.000} \\ \cline{2-5} 
                              & cov@20                & *0.0052{\textpm}0.000            & \underline{0.6709{\textpm}0.000}    & \textbf{0.9584{\textpm}0.000} \\ \hline
\multirow{4}{*}{Mindreader}   & ndcg@20               & \underline{0.069{\textpm}0.003} & \textbf{0.077{\textpm}0.004}    & *0.066{\textpm}0.001            \\ \cline{2-5} 
                              & recall@20             & \underline{0.148{\textpm}0.008} & \textbf{0.155{\textpm}0.009}    & *0.138{\textpm}0.005            \\ \cline{2-5} 
                              & precision@20          & \underline{0.016{\textpm}0.001} & \textbf{0.017{\textpm}0.000}    & *0.014{\textpm}0.000            \\ \cline{2-5} 
                              & cov@20                & *0.082{\textpm}0.005            & \underline{0.533{\textpm}0.077} & \textbf{0.561{\textpm}0.028}    \\ \hline
\multirow{4}{*}{Lastfm}       & ndcg@20               & *0.095{\textpm}0.000            & \underline{0.199{\textpm}0.000} & \textbf{0.212{\textpm}0.000}    \\ \cline{2-5} 
                              & recall@20             & *0.151{\textpm}0.000            & \underline{0.313{\textpm}0.000} & \textbf{0.319{\textpm}0.000}    \\ \cline{2-5} 
                              & precision@20          & *0.028{\textpm}0.000            & \underline{0.057{\textpm}0.000} & \textbf{0.058{\textpm}0.000}    \\ \cline{2-5} 
                              & cov@20                & *0.027{\textpm}0.000            & \textbf{0.843{\textpm}0.000}    & \underline{0.553{\textpm}0.000} \\ \hline
\multirow{4}{*}{Amazon-book}  & ndcg@20               & *0.017{\textpm}0.000            & \textbf{0.048{\textpm}0.000}    & \underline{0.037{\textpm}0.000} \\ \cline{2-5} 
                              & recall@20             & *0.036{\textpm}0.000            & \textbf{0.094{\textpm}0.000}    & \underline{0.073{\textpm}0.000} \\ \cline{2-5} 
                              & precision@20          & *0.004{\textpm}0.000            & \textbf{0.012{\textpm}0.000}    & \underline{0.009{\textpm}0.000} \\ \cline{2-5} 
                              & cov@20                & *0.003{\textpm}0.000            & \textbf{0.629{\textpm}0.000}    & \underline{0.063{\textpm}0.000} \\ \hline
\end{tabular}}
\end{table*}
